# Supplementary material for: Weakly Supervised Human-Object Interaction Detection in Video via Contrastive Spatiotemporal Regions
Source: arXiv:2110.03562 source file (2021-10-07)
Supplement: Supplementary file 2 [file result.tex]

\section{Additional experimental results}
\label{sec:additional_results}

In \fig{fig:retrieval_result} of this supplement, we show the \textbf{Rel (ko)} detection results of the proposed weakly supervised method.
As described in Section 5.1 in the main paper, 
\textbf{Rel} represents the \textbf{relation} accuracy, \ie both the predicted human and object bounding boxes match the ground truth human and object bounding boxes, respectively.    
\textbf{ko} represents the \textbf{Known Object} setting, \ie, given a human-object interaction category, we evaluate the human and object detection only on video frames containing the target human-object interaction category. 
% (\textbf{def} is more challenging because it evaluates the human and object detection on all video frames on the full test set. Here we only show the \textbf{ko} result).

As shown in \fig{fig:retrieval_result}, given a verb-object class, we select the top-detected human-object bounding boxes on our dataset and rank them based on their detection scores.
In each frame, the yellow bounding box represents the predicated human bounding box while the blue bounding box is the predicated object bounding box.
For each example, we show the positives among the top-detected pairs (green frames) and top-scored incorrect pairs (red frames).
A pair of boxes is considered as positive if both the human and object candidates overlap with the corresponding human and object ground truth with IoU $\geq$ 0.5.

In \fig{fig:retrieval_result2}, we show the \textbf{Phr (ko)} detection results of the proposed weakly supervised method.
\textbf{Phr} represents the \textbf{phrase} accuracy, \ie the union of the detected human and object bounding boxes matches the union of the ground truth human and object boxes.  

Given a verb-object class, we select the top-detected human-object bounding boxes on our dataset and rank them based on their detection scores.
In each frame, the blue bounding box represents the union of predicated human and object bounding boxes.
For each example, we show the positives among the top-detected pairs (green frames) and top-scored incorrect pairs (red frames).
A pair of boxes is considered as positive if the union of the human and object candidates overlap with the union of human and object ground truth with IoU $\geq$ 0.5.

\begin{figure*}[t]
\begin{center}
\includegraphics[width=1\linewidth]{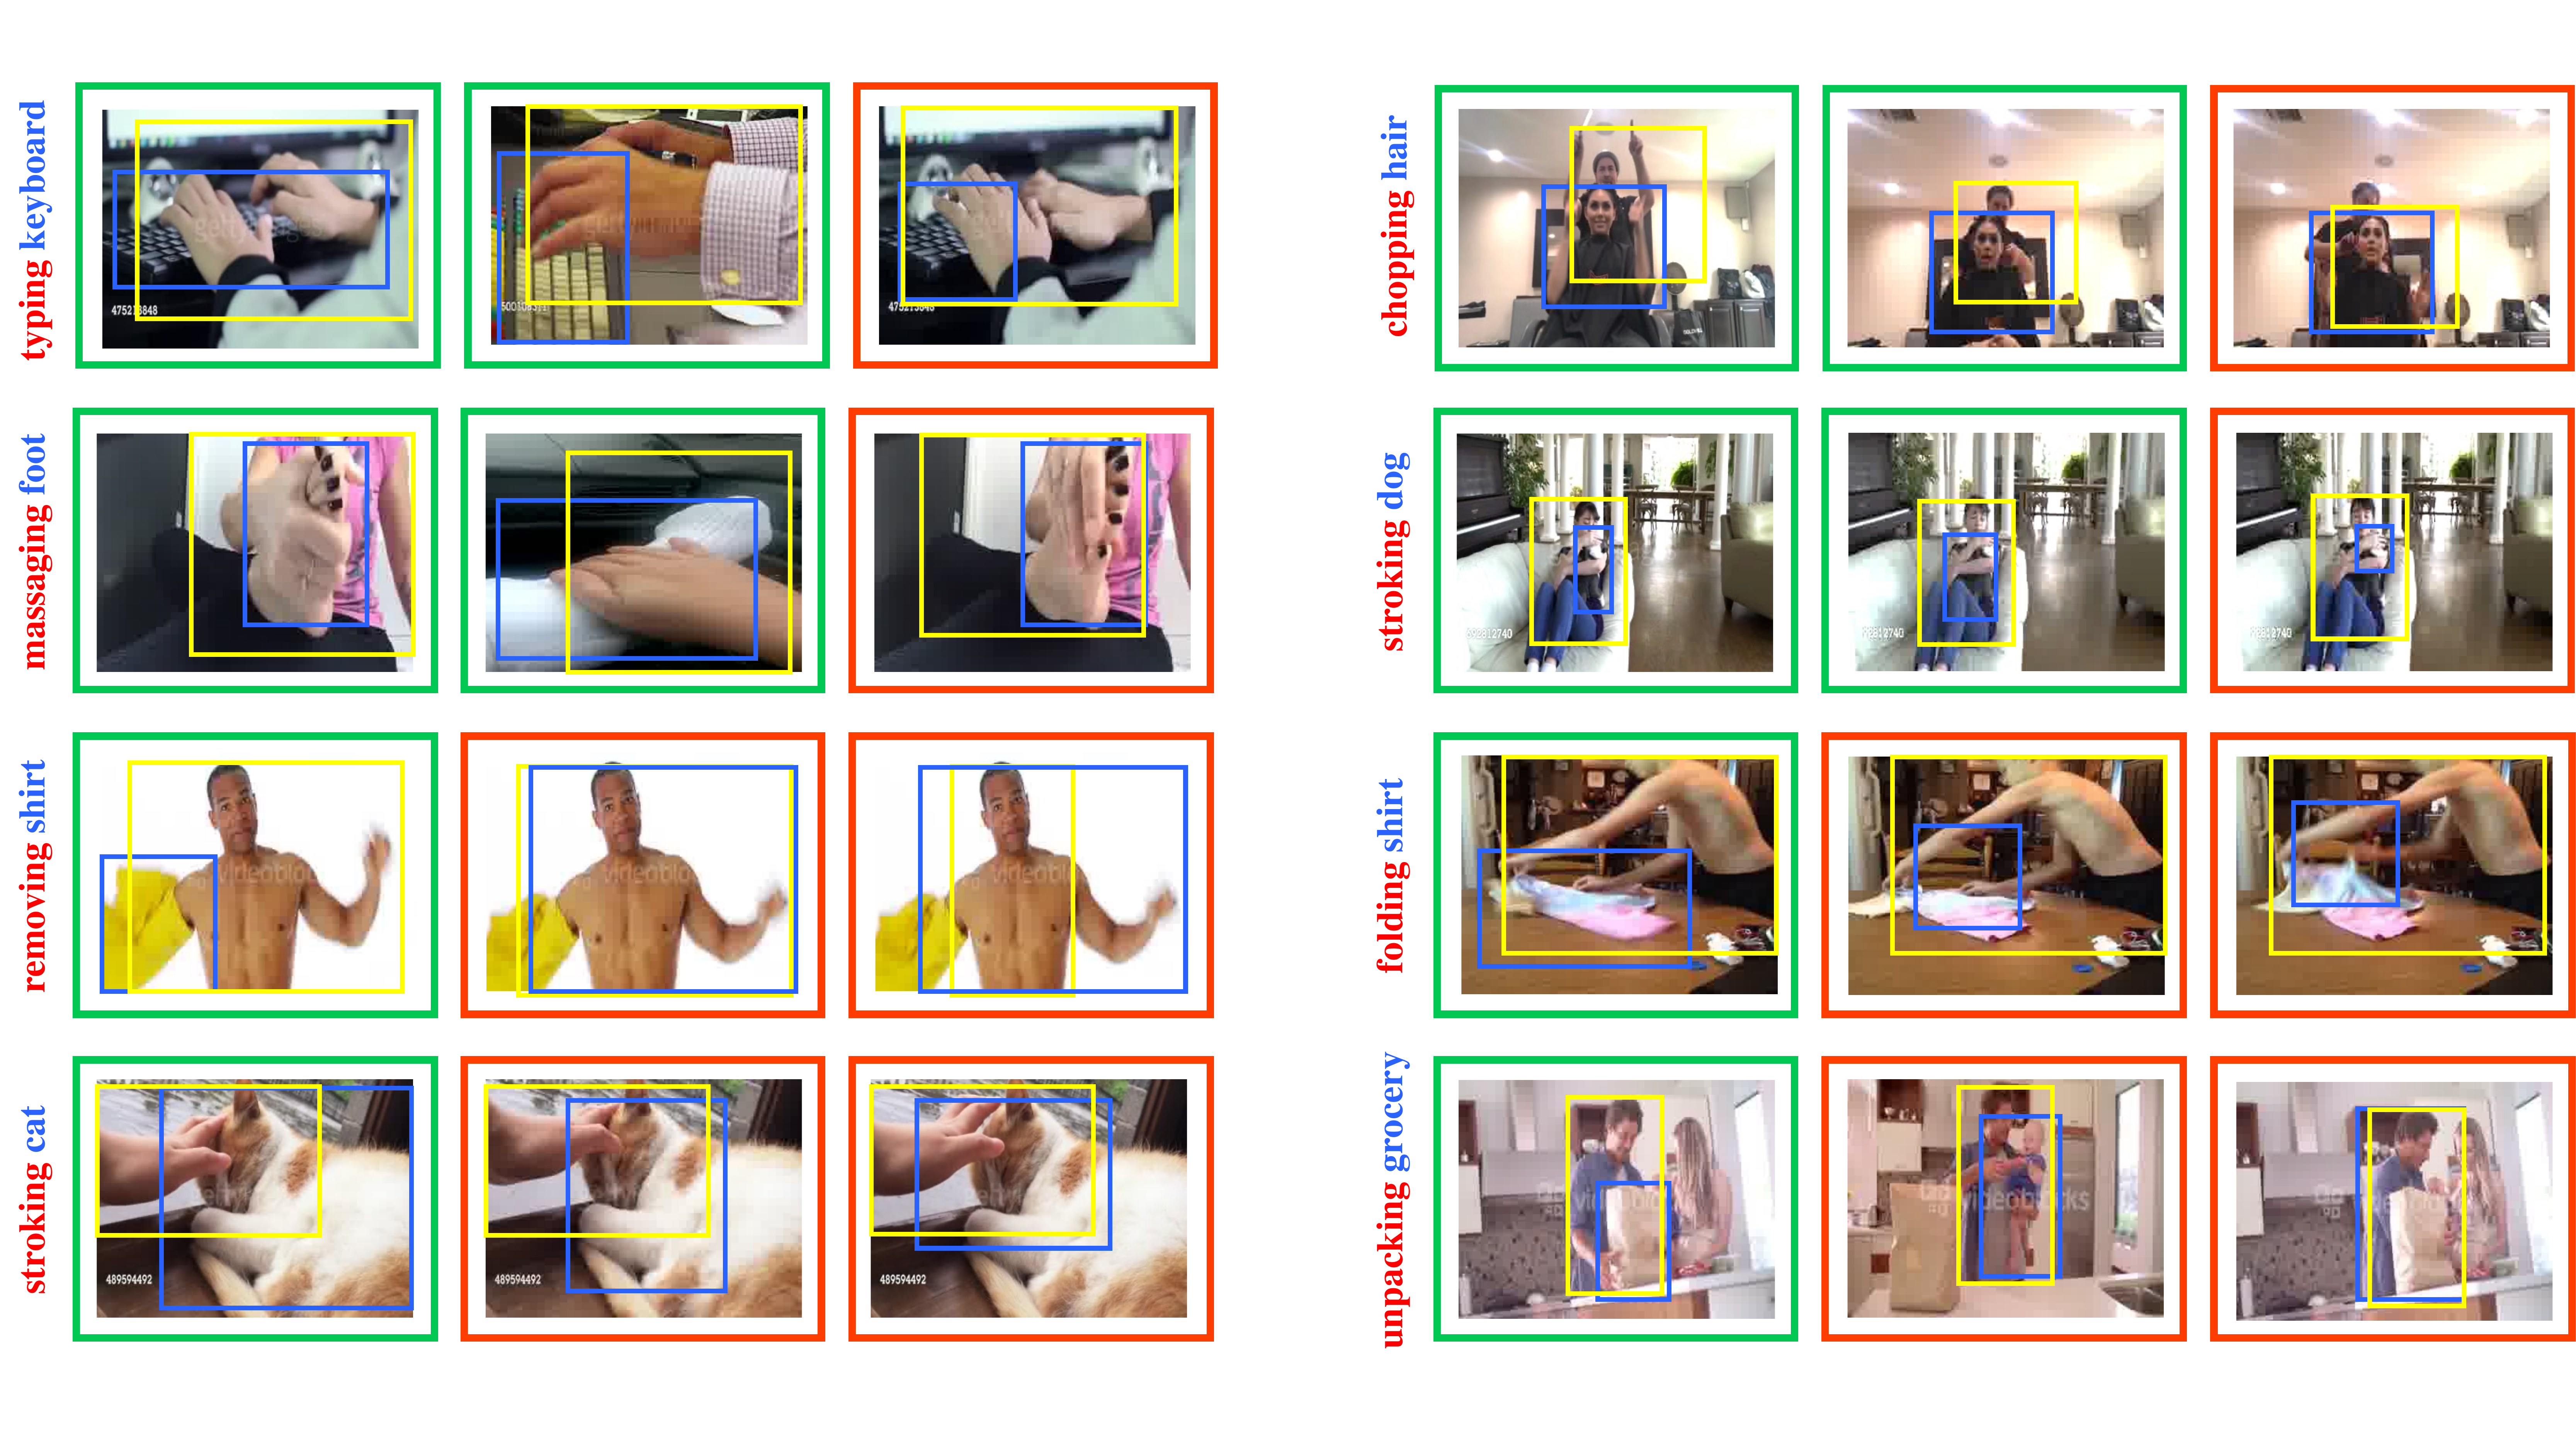}
\end{center}
\vspace{-15pt}
\caption{\small \textbf{Human-object interaction detection results.}
Given a verb-object class, we show the top-detected human-object bounding boxes on our dataset and rank them based on their detection scores.
In each frame, the yellow bounding box represents the predicated human bounding box while the blue bounding box is the predicated object bounding box.
For each example, we show the positives among the top-detected pairs (green frames) and top-scored incorrect pairs (red frames).
These results were computed using our weakly supervised method.
A pair of boxes is considered as positive if both the human and object candidates overlap with the corresponding human and object ground truth with IoU $\geq$ 0.5.
% Both the predicted human bounding box object bounding box match the ground truth 'ko'. 
}
\label{apx_fig:retrieval_result}
\end{figure*}

\begin{figure*}[t]
\begin{center}
\includegraphics[width=1\linewidth]{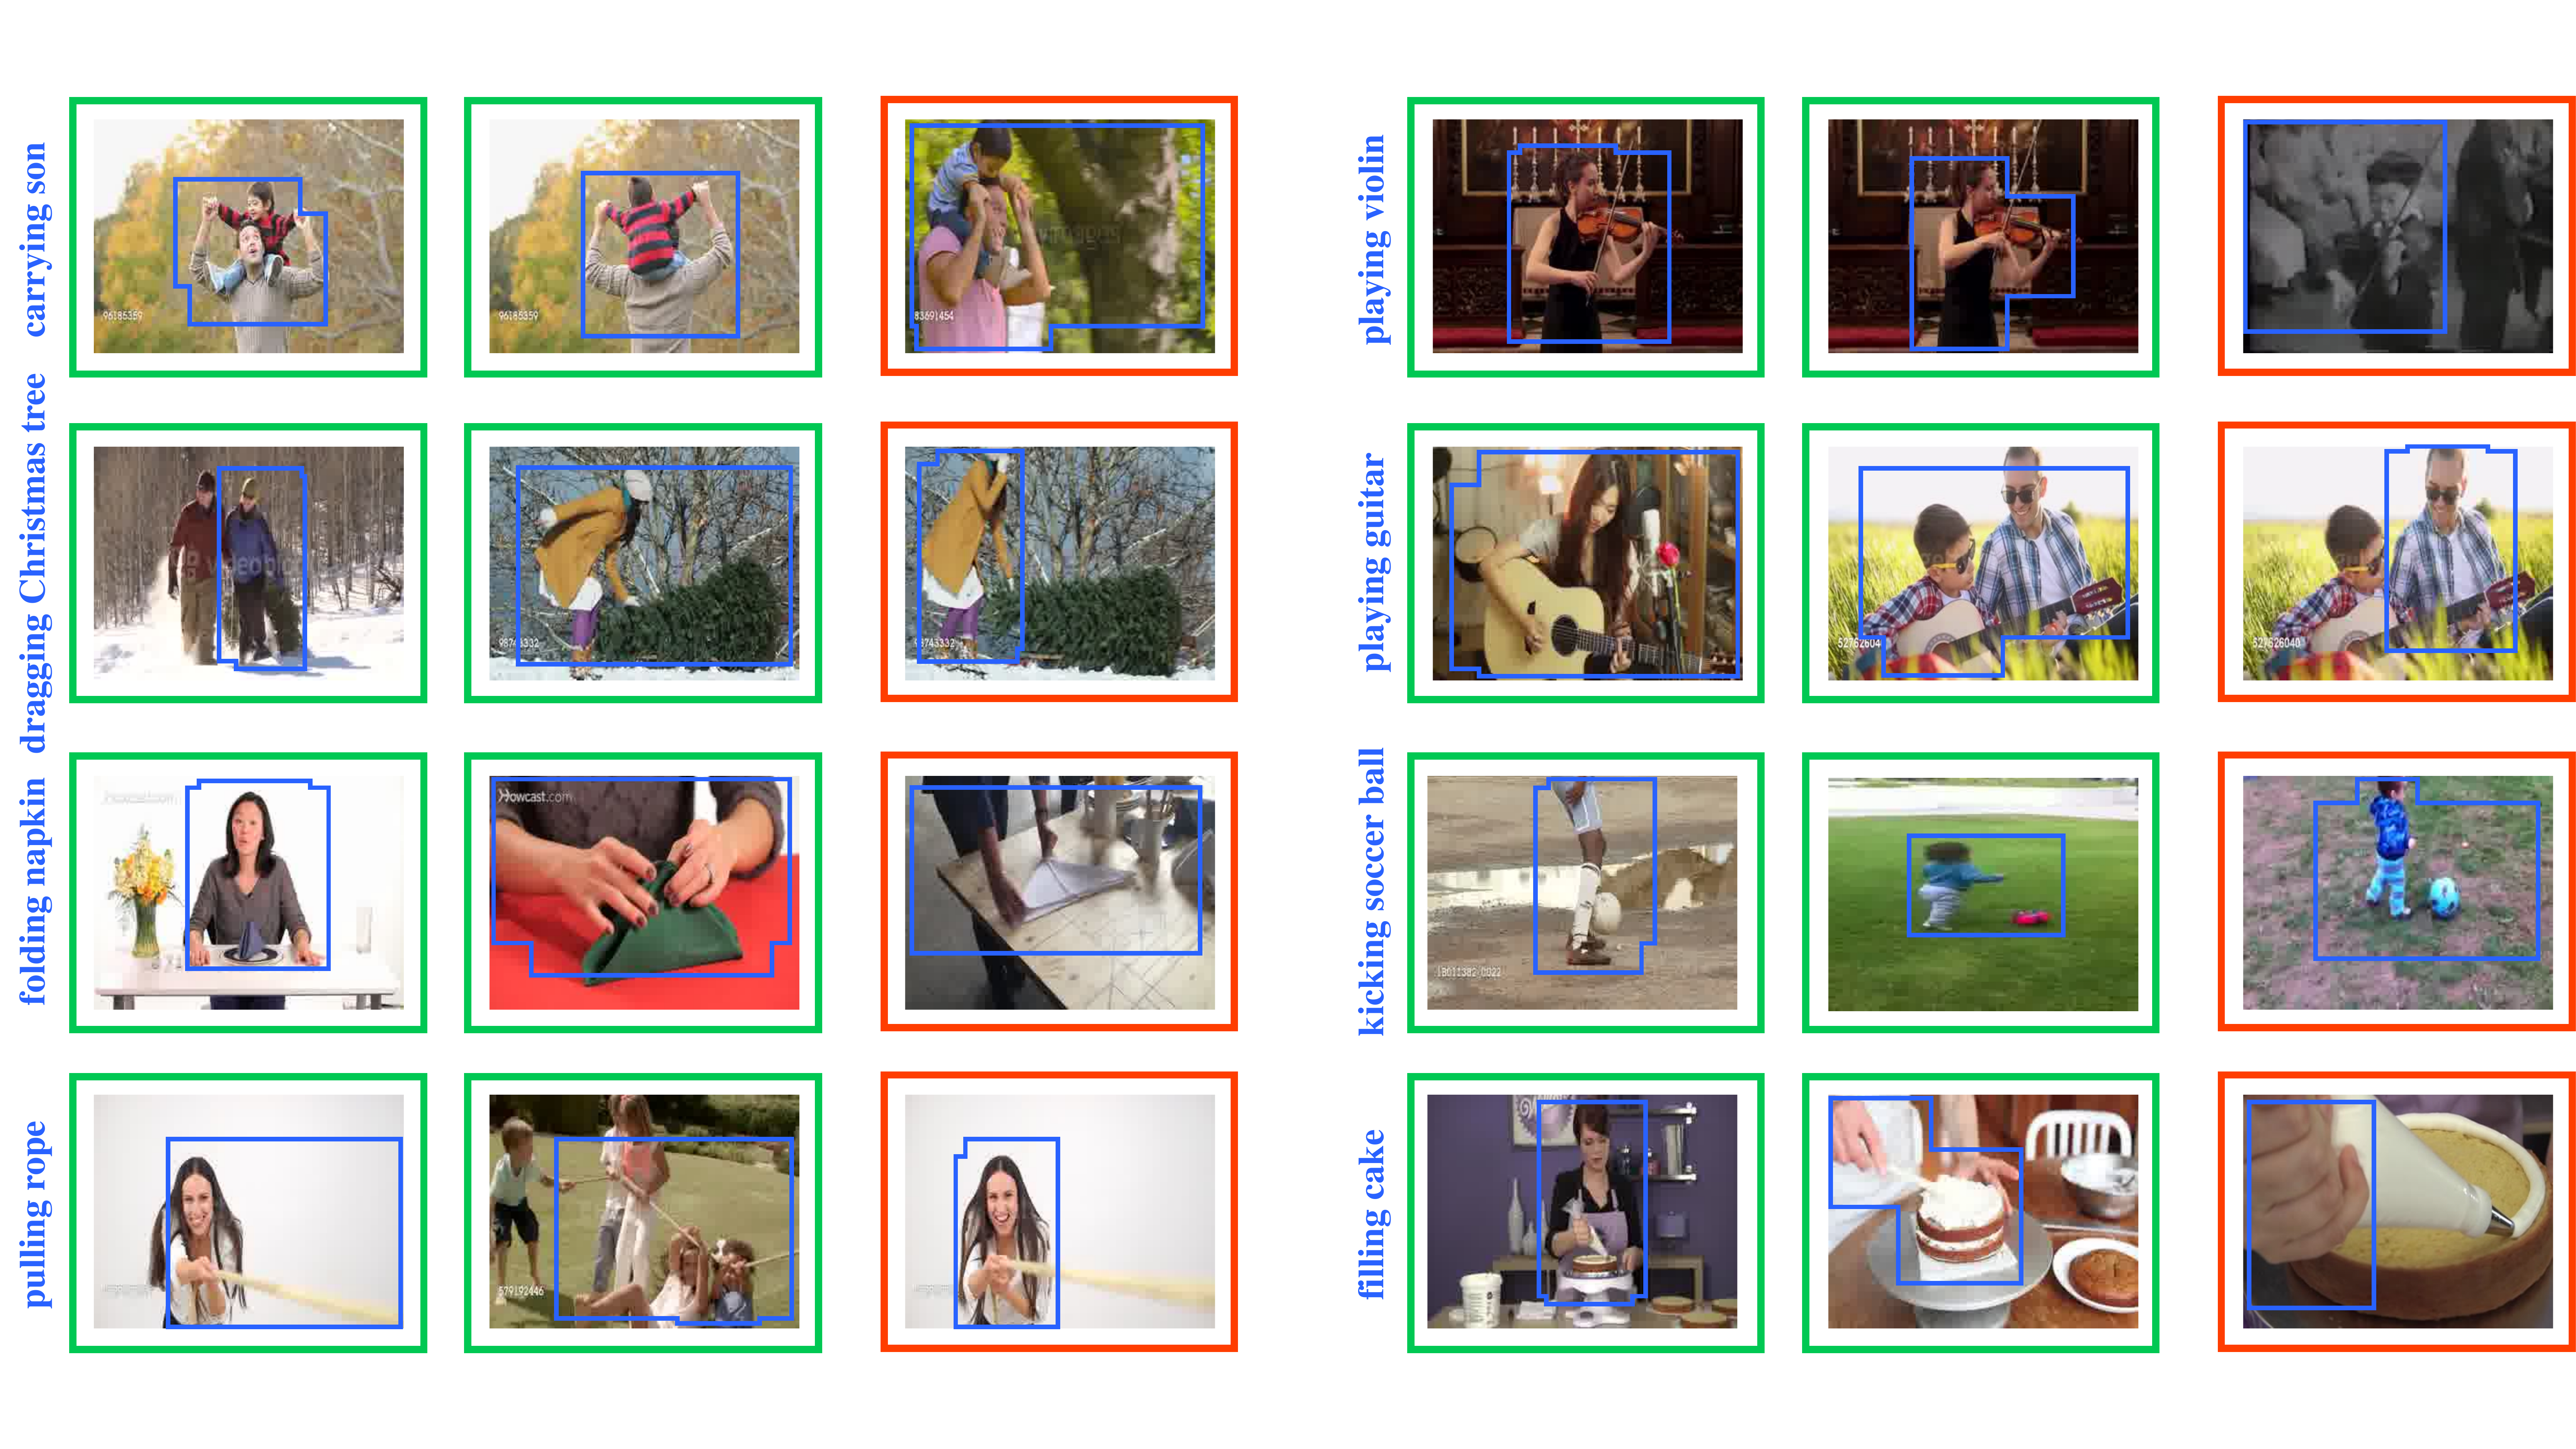}
\end{center}
\vspace{-15pt}
\caption{\small \textbf{Human-object interaction detection results.}
Given a verb-object class, we show the top-detected human-object bounding boxes on our dataset and rank them based on their detection scores.
In each frame, the blue bounding box represents the union of predicated human and object bounding boxes.
For each example, we show the positives among the top-detected pairs (green frames) and top-scored incorrect pairs (red frames).
These results were computed using our weakly supervised method.
A pair of boxes is considered as positive if the union of the human and object candidates overlap with the union of human and object ground truth with IoU $\geq$ 0.5.
}
\label{apx_fig:retrieval_result2}
\vspace{-10pt}
\end{figure*}
