# Supplementary material for: Weakly Supervised Human-Object Interaction Detection in Video via Contrastive Spatiotemporal Regions
Source: arXiv:2110.03562 source file (2021-10-07)
Supplement: Supplementary file 3 [file retrieval_result.tex]

\begin{figure*}[t]
\begin{center}
\includegraphics[width=1\linewidth]{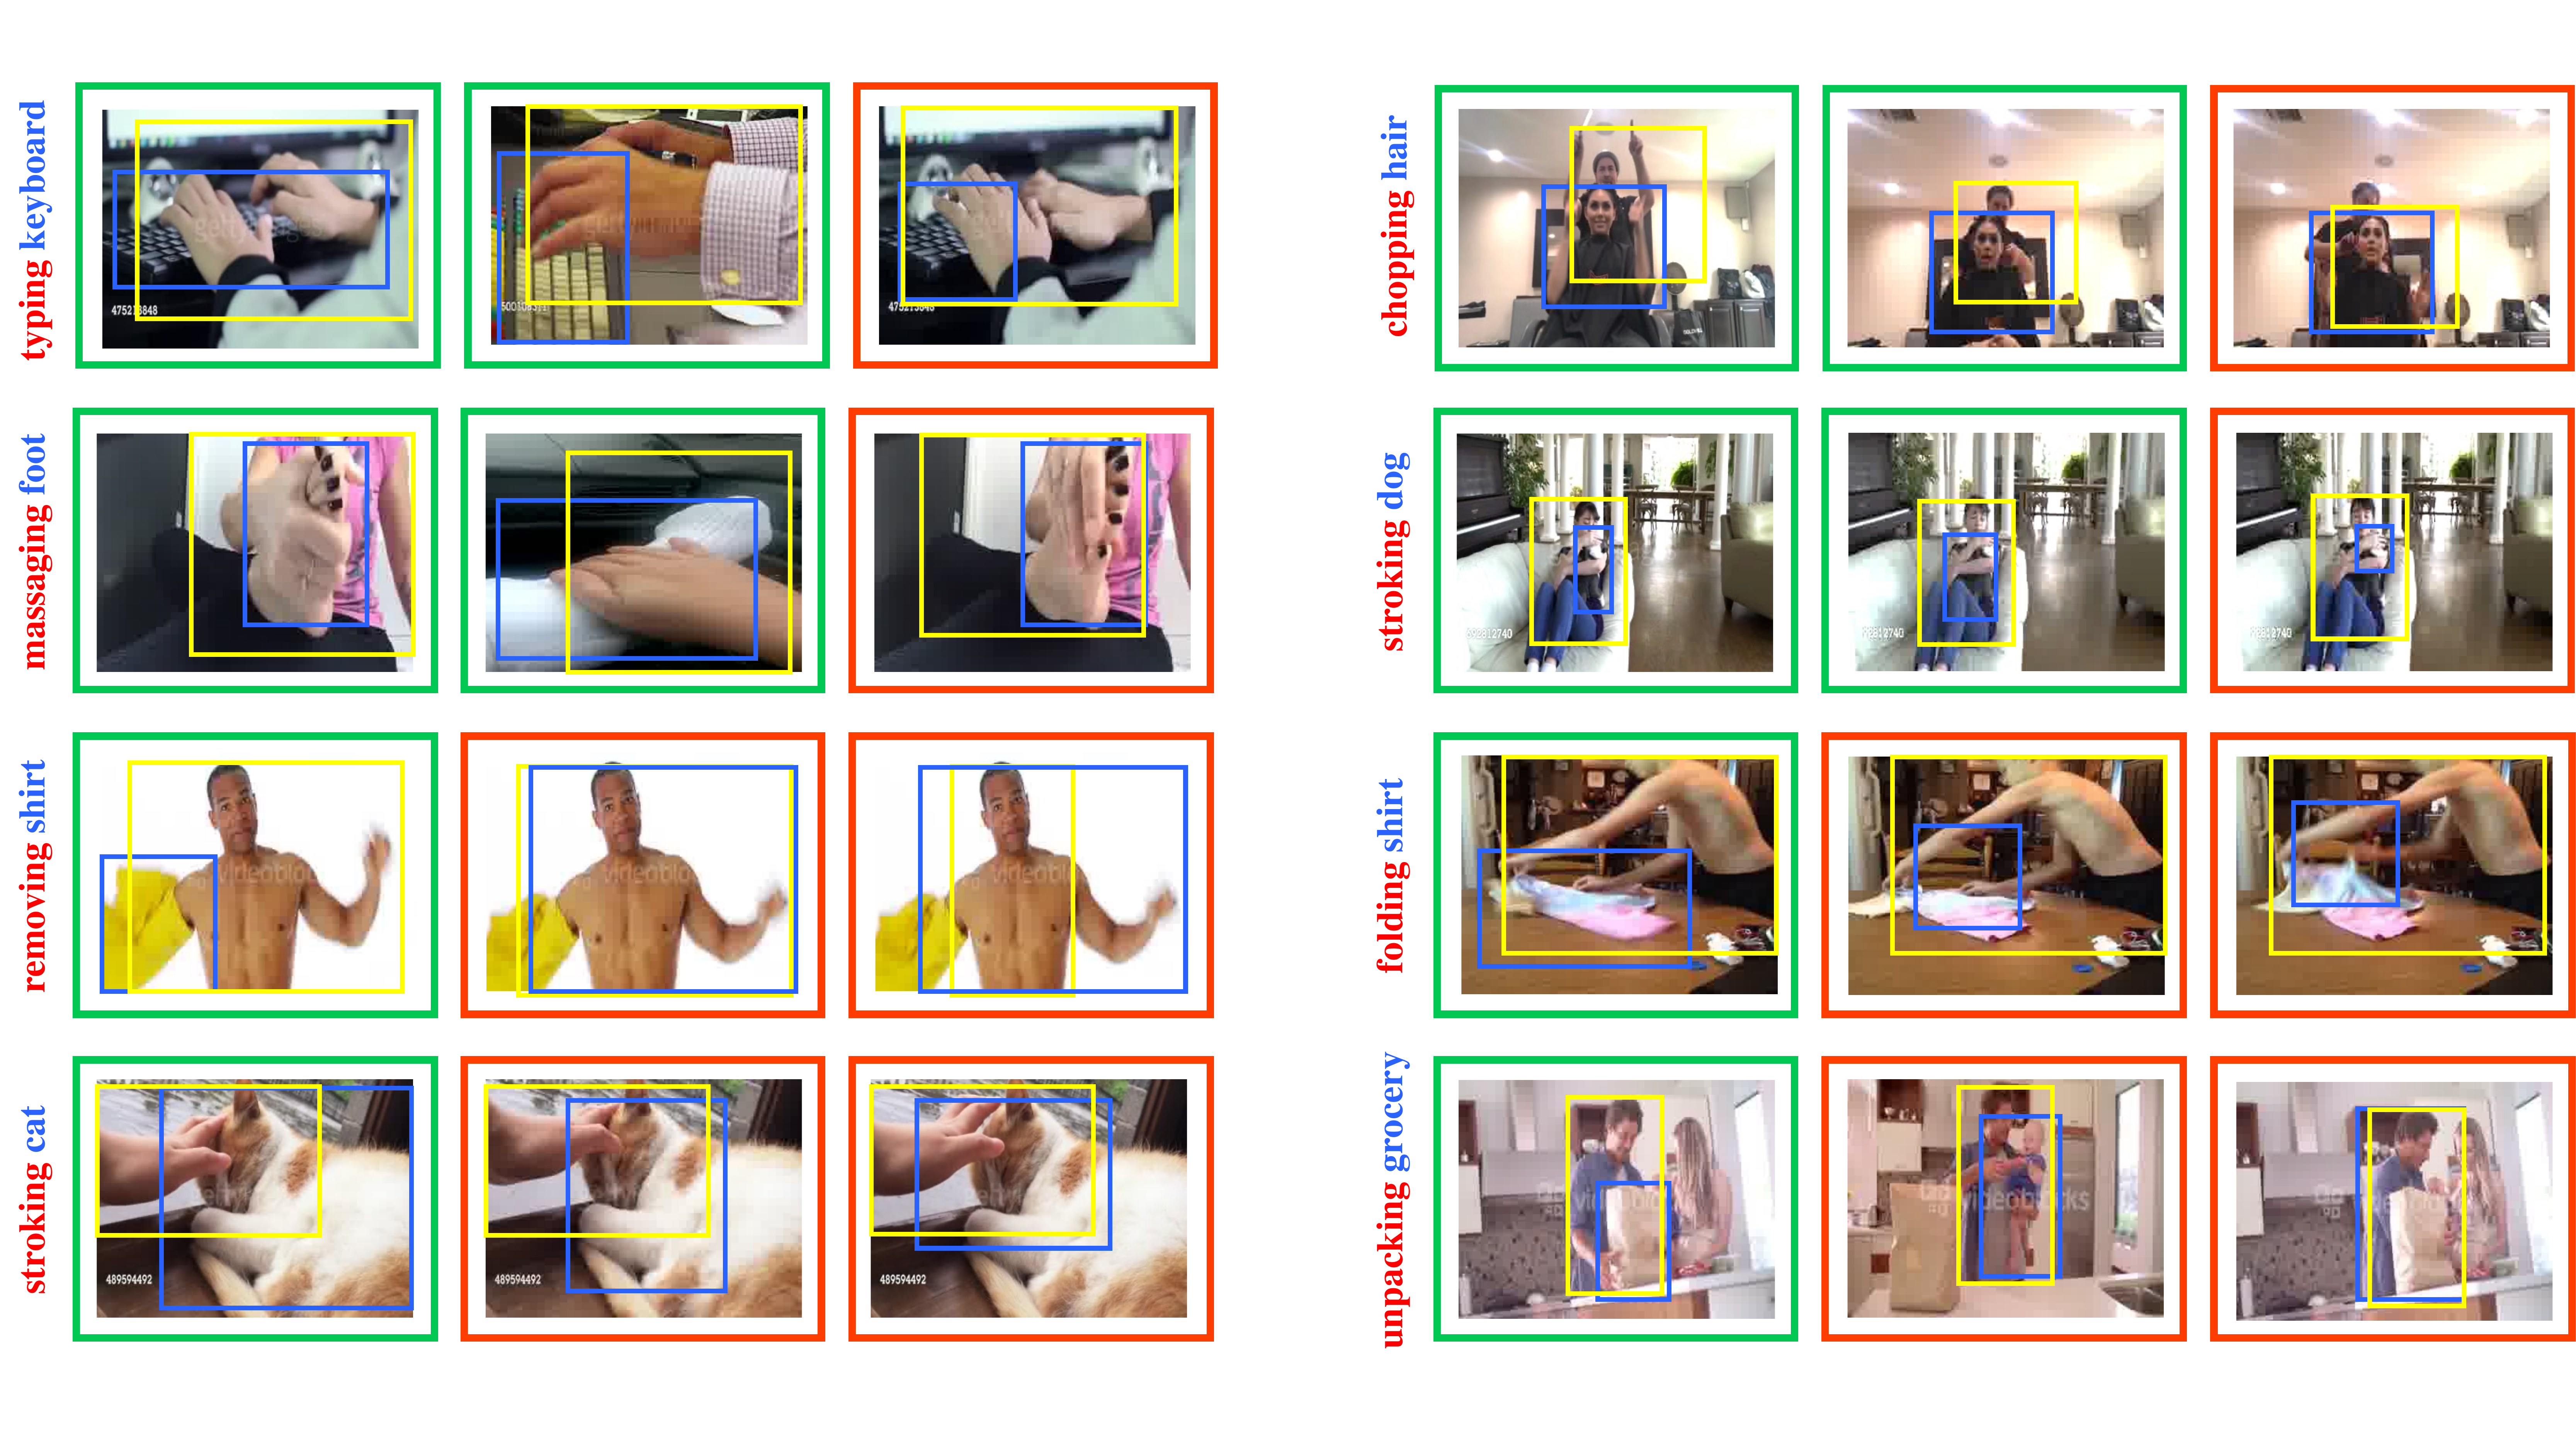}
\end{center}
\vspace{-15pt}
\caption{\small \textbf{Human-object interaction detection results.}
Given a verb-object class, we show the top-detected human-object bounding boxes on our dataset and rank them based on their detection scores.
In each frame, the yellow bounding box represents the predicated human bounding box while the blue bounding box is the predicated object bounding box.
For each example, we show the positives among the top-detected pairs (green frames) and top-scored incorrect pairs (red frames).
These results were computed using our weakly supervised method.
A pair of boxes is considered as positive if both the human and object candidates overlap with the corresponding human and object ground truth with IoU $\geq$ 0.5.
% Both the predicted human bounding box object bounding box match the ground truth 'ko'. 
}
\label{apx_fig:retrieval_result}
\end{figure*}

\begin{figure*}[t]
\begin{center}
\includegraphics[width=1\linewidth]{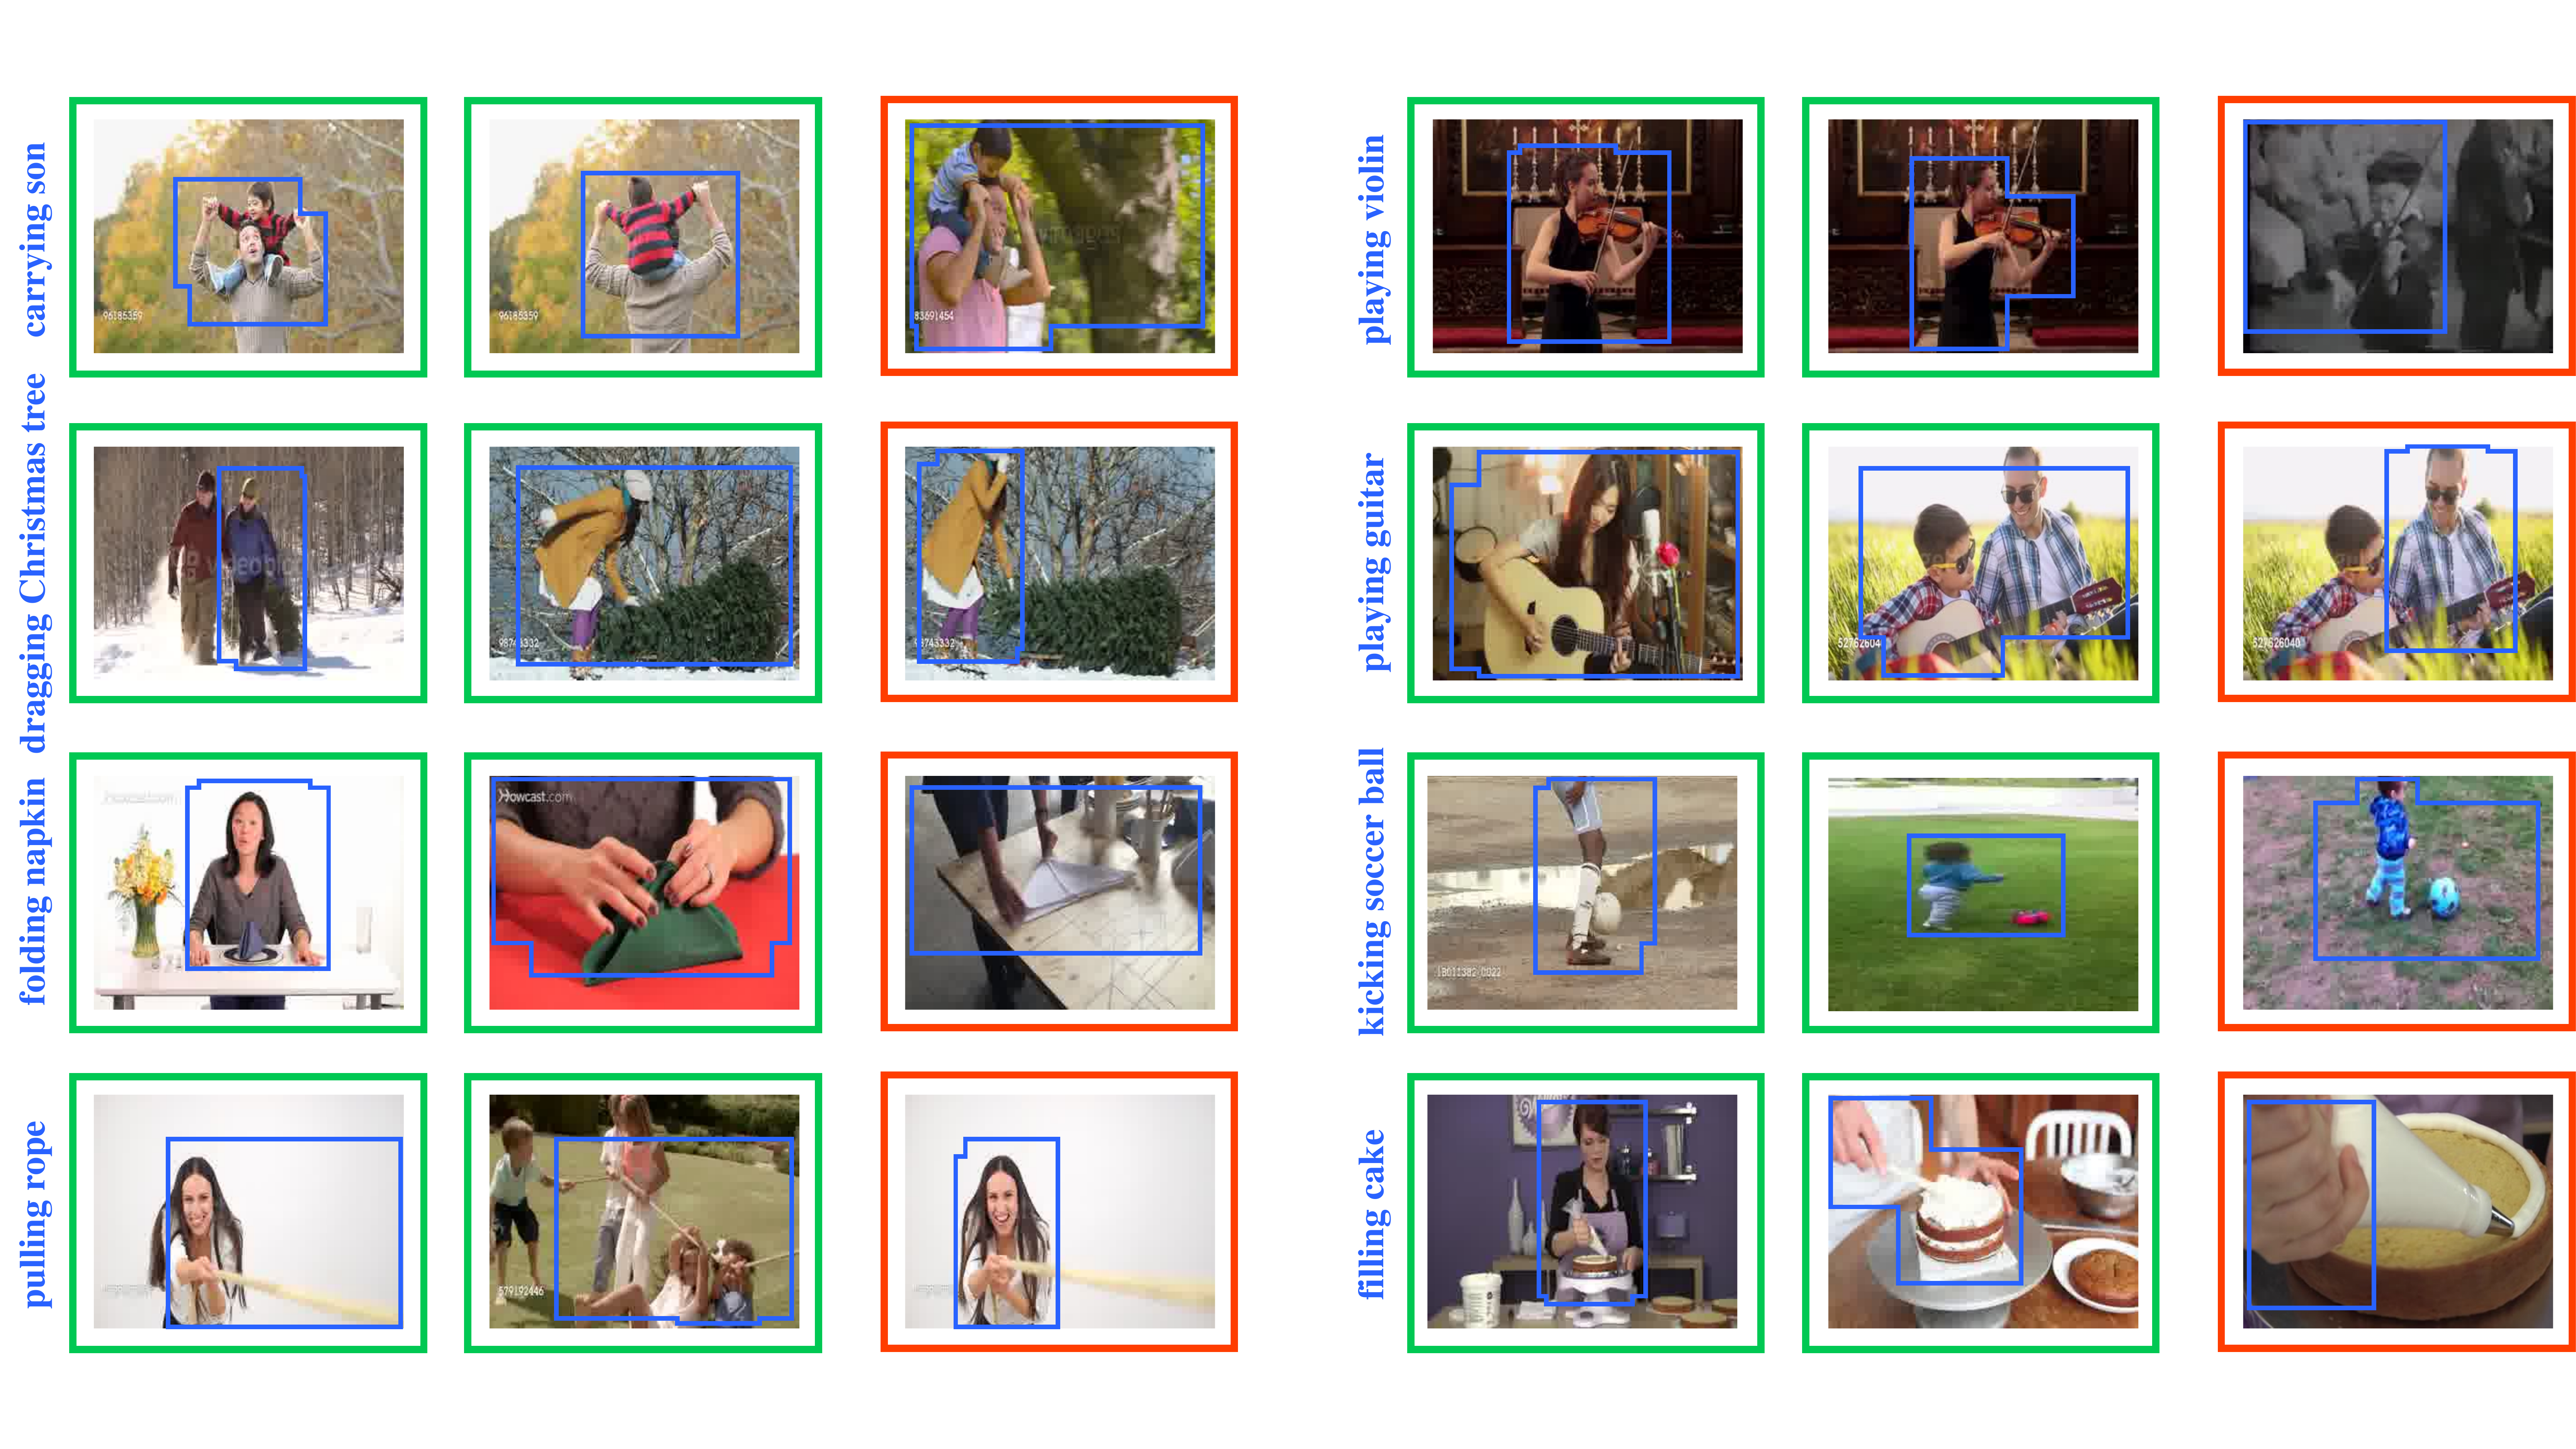}
\end{center}
\vspace{-15pt}
\caption{\small \textbf{Human-object interaction detection results.}
Given a verb-object class, we show the top-detected human-object bounding boxes on our dataset and rank them based on their detection scores.
In each frame, the blue bounding box represents the union of predicated human and object bounding boxes.
For each example, we show the positives among the top-detected pairs (green frames) and top-scored incorrect pairs (red frames).
These results were computed using our weakly supervised method.
A pair of boxes is considered as positive if the union of the human and object candidates overlap with the union of human and object ground truth with IoU $\geq$ 0.5.
}
\label{apx_fig:retrieval_result2}
\vspace{-10pt}
\end{figure*}
