# Supplementary material for: Weakly Supervised Human-Object Interaction Detection in Video via Contrastive Spatiotemporal Regions
Source: arXiv:2110.03562 source file (2021-10-07)
Supplement: Supplementary file 4 [file othermethods.tex]

\begin{table*}[t]
\footnotesize
\caption{\small Evaluation of performance on \lsdata compared to methods in \cite{peyre2017weakly}, \cite{zhou2018weakly}, \cite{xiao2020visual} and different random baselines. Phrase (Phr) detection refers to correct localization (0.5 IoU) of the union of human and object bounding boxes while relationship (Rel) refers to correct localization of both human and object bounding boxes. (ko) and (def) are the known object setting and default setting.}
\vspace{-15pt}
\label{tbl:other}
\begin{center}
\setlength{\tabcolsep}{5pt}
\resizebox{0.9\textwidth}{!}{
\begin{tabular}{c|cccc|cc|cc|cc}
\toprule
\bf Model & \multicolumn{4}{c|}{\bf mAP (\%)} & \multicolumn{2}{c|}{\bf Recall@1 (\%)} & \multicolumn{2}{c|}{\bf Video One Recall@1 (\%)} & \multicolumn{2}{c}{\bf Video All Recall@1 (\%)}  \\
\midrule
\midrule
& Phr (ko) & Phr (def) & Rel (ko) & Rel (def) &  Phr & Rel & Phr & Rel & Phr & Rel \\
\midrule
Ours Random & 7.27 & 0.02 & 0.03 & 0.00 &	22.78 & 0.23 & 38.44 & 0.72 & 3.53 & 0.00 \\
Ours Random Pretrain & 7.04 & 0.02 & 0.00 & 0.00 & 23.22 & 0.37 & 40.06 & 2.01 & 3.90 & 0.00 \\
% Peyre2017 \cite{peyre2017weakly} & 23.34 & 0.31 & 0.21 & 0.00 & 33.69 & 0.97 & 66.23 & 2.87 & 7.31 & 0.21 \\
% Peyre2017 \cite{peyre2017weakly} & 27.98 & 0.43 & 0.28 & 0.00 & 33.69 & 0.97 & 66.23 & 2.87 & 7.31 & 0.21 \\
Peyre2017 \cite{peyre2017weakly} & 27.98 & \bf 0.43 & 0.28 & 0.00 & 37.64 & 1.01 & 61.66 & 2.52 & 13.34 & 0.24 \\
% Zhou2018 \cite{zhou2018weakly} & 7.96 & 0.02 & 0.08 & 0.00 & 48.39 & 2.13 & 74.67 & 5.88 & 23.65 & 0.00 \\
Zhou2018 \cite{zhou2018weakly} & 11.96 & 0.22 & 0.16 & 0.00 & 48.39 & 2.13 & 74.67 & 5.88 & 23.65 & 0.00 \\
% Zhou2018 \cite{zhou2018weakly} & 11.96 & 0.22 & 0.16 & 0.00 & 15.13 & 0.14 & 28.73 & 0.24 & 3.73 & 0.00 \\
% Xiao2020 \cite{xiao2020visual} & 12.31 & 0.04 & 0.99 & 0.01 \\
Xiao2020 \cite{xiao2020visual} & 27.09 & 0.09 & 1.42 & 0.00 & 36.80 & 1.86 & 50.60 & 3.61 & 22.53 & 0.60 \\
\midrule
Ours+Npair & 39.84 &  0.42 & 6.42 & 0.08 & 64.25 & \bf 13.78 & 80.94 & \bf 28.06 & 46.16 & 3.72 \\
Ours+Con & \bf 45.91 & 0.38 & \bf 9.37 & \bf 0.09 & \bf 67.18 & 13.72 & \bf 84.38 & 27.40 & \bf 49.52 & \bf 4.09 \\
\bottomrule
\end{tabular}
}
\end{center}
\end{table*}
