# Supplementary material for: Weakly Supervised Human-Object Interaction Detection in Video via Contrastive Spatiotemporal Regions
Source: arXiv:2110.03562 source file (2021-10-07)
Supplement: Supplementary file 5 [file unseen.tex]

\begin{table*}[t]
\footnotesize
\caption{\small Evaluation of various models on the unseen test set on \lsdata. The unseen test set consists of 53 classes of objects unseen during training. Evaluation at IoU threshold 0.5. (ko) and (def) are the known object setting and default setting.}
\vspace{-15pt}
\label{tbl:unseen}
\begin{center}
\resizebox{0.9\textwidth}{!}{
\begin{tabular}{c|cccc|cc|cc|cc}
\toprule
\bf Model & \multicolumn{4}{c|}{\bf mAP (\%)} & \multicolumn{2}{c|}{\bf Recall@1 (\%)} & \multicolumn{2}{c|}{\bf Video One Recall@1 (\%)} & \multicolumn{2}{c}{\bf Video All Recall@1 (\%)} \\
\midrule
\midrule
& Phr (ko) & Phr (def) & Rel (ko) & Rel (def) &  Phr & Rel & Phr & Rel & Phr & Rel \\
\midrule
% Ours Random  & 1.46 & 0.39 & 0.00 & 0.00 & 3.90 & 0.65 & 7.27 & 1.82 & 0.00 & 0.00 \\
Ours Random  & 1.46 & 0.19 & 0.00 & 0.00 & 1.95 & 0.65 & 5.36 & 1.79 & 0.00 & 0.00 \\
% Ours Random  Pretrain & 2.49 & 0.06 & 0.00 & 0.00 & 4.52 & 0.00 & 7.14 & 0.00 & 1.79 & 0.00 \\
Ours Random  Pretrain & 2.49 & 0.06 & 0.00 & 0.00 & 2.61 & 0.00 & 7.27 & 0.00 & 0.00 & 0.00 \\
% Peyre2017 \cite{peyre2017weakly} & 7.07 & 0.29 & 0.08 & 0.00 & 7.10 & 0.00 & 15.38 & 0.00 & 1.79 & 0.00 \\
Peyre2017 \cite{peyre2017weakly} & 7.07 & 0.29 & 0.08 & 0.00 & 6.67 & 0.00 & 12.96 & 0.00 & 1.85 & 0.00 \\
\midrule
% Ours-npair & 5.45 & 0.44 & 1.38 & 0.22 & 10.46 & 3.27 & 16.36 & 7.27 & 5.45 & 0.00 \\
Ours+Npair & 7.14 & 0.38 & 3.99 & \bf 0.29 & 11.04 & 3.25 & 16.07 & 8.93 & \bf 5.36 & 0.00 \\
Ours+Con & \bf 9.08 & \bf 0.52 & \bf 5.33 & 0.24 & \bf 12.34 & \bf 6.49 & \bf 19.64 & \bf 10.71 & 3.58 & \bf 1.79 \\
\bottomrule
\end{tabular}
}
\end{center}
\end{table*}
